# Supplementary material for: Sizing Strategies for Algorithmic Trading in Volatile Markets: A Study of Backtesting and Risk Mitigation Analysis
Source: arXiv:2309.09094 source file (2023-09-19)
Supplement: Supplementary file 2 [file appendix_2.tex]

% ******************************* Thesis Appendix B ********************************

\chapter*{Overleaf: GitHub for \LaTeX\ projects }

This Project was developed using Overleaf(\url{https://www.overleaf.com/}), an online \LaTeX\ editor that allows real-time collaboration and online compiling of projects to PDF format. In comparison to other \LaTeX\ editors, Overleaf is a server-based application, which is accessed through a web browser.
